# Supplementary material for: A simple test for causality in complex systems
Source: arXiv:2005.01860 source file (2020-05-04)

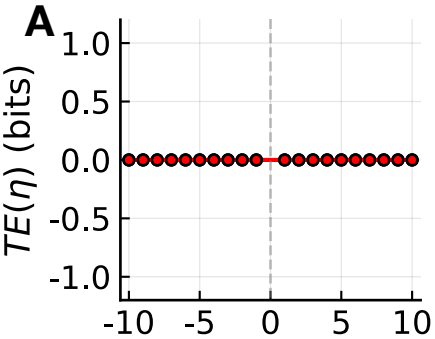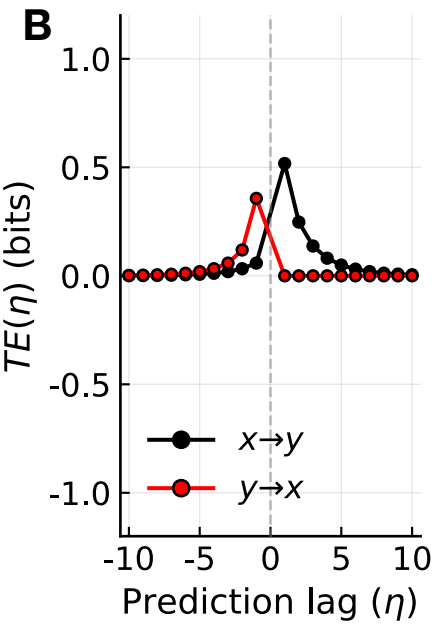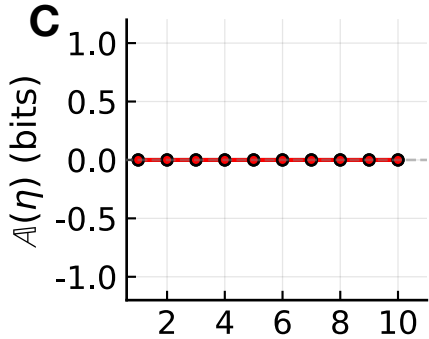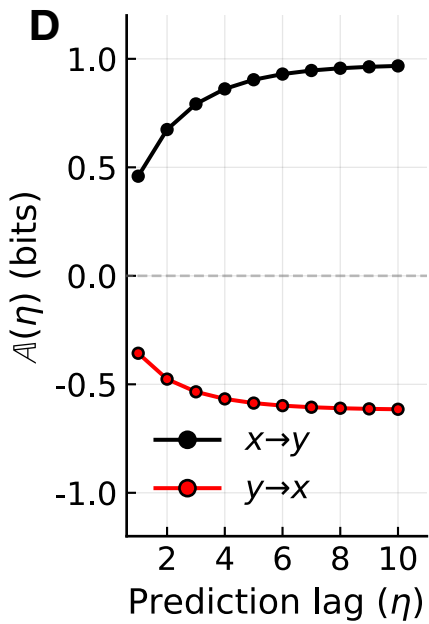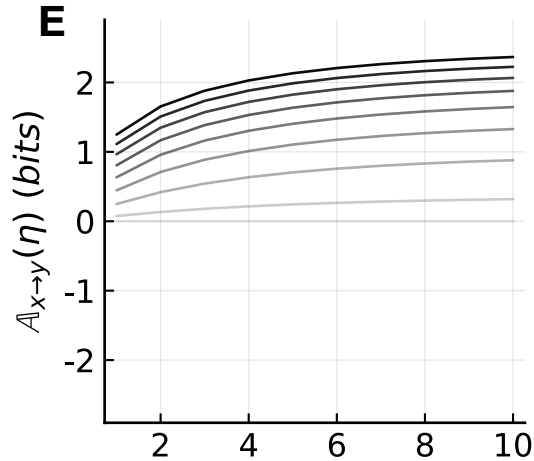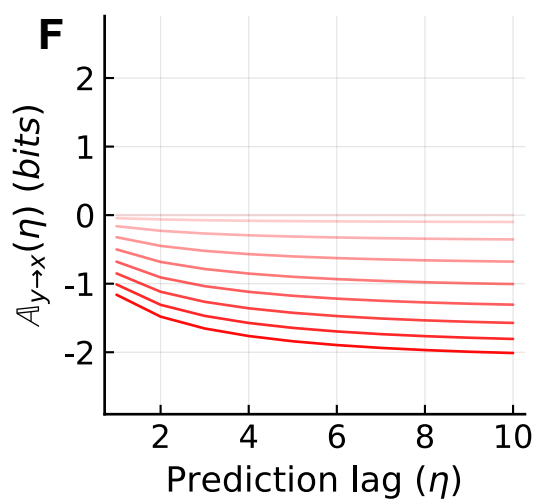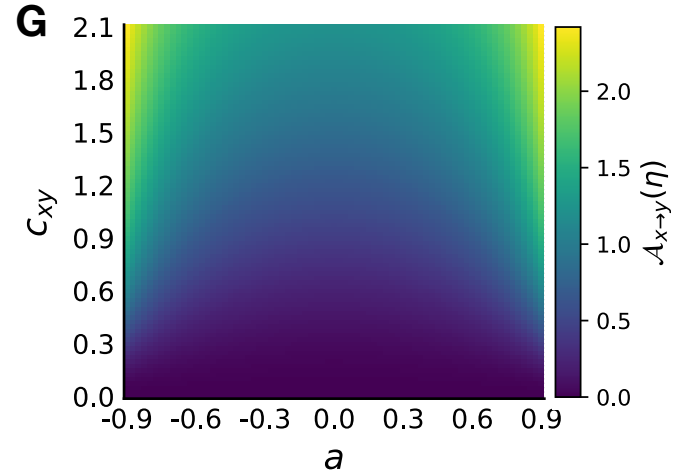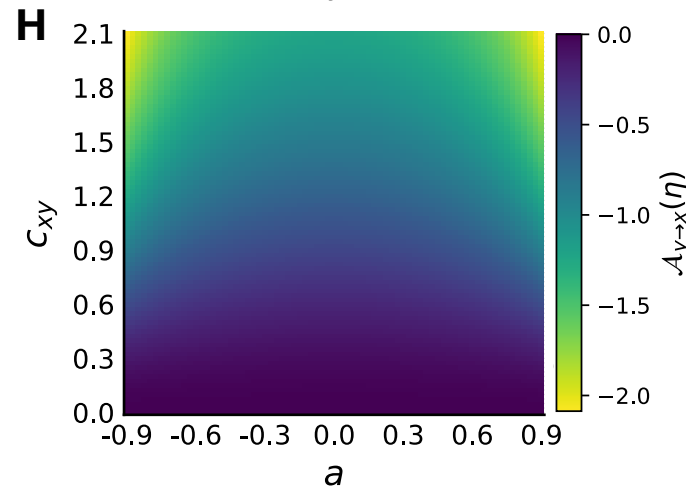

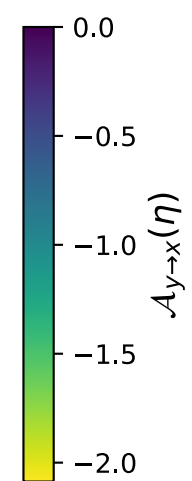

Supplement: Supplementary file 1 [file exact_asymmetries_c08_eta10.pdf]
